# Supplementary material for: Systematic derivation of hybrid coarse-grained models
Source: arXiv:1804.08157 ancillary file (2018-08-06)
Supplement: Supplementary file 1 [file SI.pdf]

# Supplemental Material for
# " Systematic derivation of hybrid coarse-grained models "

Nicodemo Di Pasquale [a]
*Department of Mathematics, University of Leicester, University Rd, Leicester LE1 7RH, UK*[†]

Thomas Hudson
*Warwick Mathematics Institute, University of Warwick, Coventry CV4 7AL, UK*[‡]

Matteo Icardi
*School of Mathematical Sciences, University of Nottingham, Nottingham NG7 2RD, UK*[§]

---

[a] Alphabetical order
[†] Email: ndp8@leicester.ac.uk
[‡] Email: t.hudson.1@warwick.ac.uk
[§] Email: matteo.icardi@nottingham.ac.uk

## I. CONDITIONAL EXPECTATION

The starting point of our analysis is the definition of the Fine-Grained phase space $X = \mathbb{R}^{6M^{FG}}$, where we write $\boldsymbol{\gamma} = (\boldsymbol{\gamma}_{\mathbf{r}}, \boldsymbol{\gamma}_{\mathbf{p}})$ to denote a vector of $3M^{FG}$ position variables $\boldsymbol{\gamma}_{\mathbf{r}}$, and $3M^{FG}$ momenta $\boldsymbol{\gamma}_{\mathbf{p}}$. Let $\mathcal{H} : X \to \mathbb{R}$ and $\beta > 0$ such that $e^{-\beta\mathcal{H}}$ is integrable with respect to the Lebesgue measure on $X$.

The Gibbs measure on $X$ is the probability measure defined to be

$$\mu(\mathrm{d}\boldsymbol{\gamma}) = \rho(\boldsymbol{\gamma})\mathrm{d}\boldsymbol{\gamma} = \frac{1}{\mathcal{Z}}\mathbf{e}^{-\beta\mathcal{H}(\boldsymbol{\gamma})}\mathrm{d}\boldsymbol{\gamma} \tag{S.1}$$

As a consequence of Liouville's Theorem, the Gibbs measure is invariant under the flow generated by Hamilton's equations of motion. The flow $\boldsymbol{\eta}^t : X \to X$ of an Hamiltonian system is the mapping that moves the solution ahead of a time $t$. The point $\boldsymbol{\eta}^t(\boldsymbol{\gamma}_0) = (\boldsymbol{\gamma}_1(\boldsymbol{\gamma}_0; t), \ldots, \boldsymbol{\gamma}_{6M^{FG}}(\boldsymbol{\gamma}_0; t))$ is the point of the trajectory which corresponds to solution with initial conditions $\boldsymbol{\gamma}_0$. The system eq. (1) can be rewritten as:

$$\frac{\mathrm{d}\boldsymbol{\eta}^t}{\mathrm{d}t} = \mathbf{b}(\boldsymbol{\eta}^t(\boldsymbol{\gamma}_0)), \qquad \boldsymbol{\eta}^0(\boldsymbol{\gamma}) = \boldsymbol{\gamma}_0,$$

where $\mathbf{b} : X \to \mathbb{R}^{6M^{FG}}$, $\mathbf{b}(\boldsymbol{\gamma}) = \boldsymbol{\Lambda}\frac{\partial\mathcal{H}(\boldsymbol{\gamma})}{\partial\boldsymbol{\gamma}}$ represents the Hamiltonian vector field.

In the FG space we define *phase functions* $A : X \to \mathbb{R}$ satisfying $A \in L^2(X;\mu)$. If $L^2(X;\mu)$ is equipped with the usual scalar product

$$(A, B) = \int A(\boldsymbol{\gamma})B(\boldsymbol{\gamma})\mu(\mathrm{d}\boldsymbol{\gamma}) = \int A(\boldsymbol{\gamma})B(\boldsymbol{\gamma})\rho(\boldsymbol{\gamma})\mathrm{d}\boldsymbol{\gamma}, \tag{S.2}$$

$L^2(X;\mu)$ is a Hilbert space. Phase functions evolve in time because of the time evolution of phase variables under the Hamiltonian flow. The evolution of phase function is described by the Liouville equation eq. (2) which we rewrite here using the new notation defined in this section:

$$\frac{\mathrm{d}A^t(\boldsymbol{\gamma})}{\mathrm{d}t} = \mathfrak{L}A^t(\boldsymbol{\gamma}) \qquad A^0(\boldsymbol{\gamma}) = A(\boldsymbol{\gamma}) \tag{S.3}$$

where $\mathfrak{L}$ is the Liouville operator defined in eq. (2), $\mathfrak{L} := \mathbf{b}(\boldsymbol{\gamma}) \cdot \frac{\partial}{\partial\boldsymbol{\gamma}}$. Using the definition of $\boldsymbol{\eta}^t$, the solution of eq. (S.3) is $A^t(\boldsymbol{\gamma}) = A(\boldsymbol{\eta}^t(\boldsymbol{\gamma}))$[1].

If we suppose that the state of the system is described by the equilibrium distribution $\rho(\boldsymbol{\gamma})$, the observed value of the phase function $A \in L^2(X;\mu)$ is the expected value with respect to the measure $\mu$:

$$\mathbb{E}[A] = \int A(\boldsymbol{\gamma})\mu(\mathrm{d}\boldsymbol{\gamma}). \tag{S.4}$$

$A$ may therefore be considered a random variable. We now focus our attention on a set of functions $A_I \in L^2(X;\mu)$, with $I = 1, \ldots, M^{CG}$ and $M^{CG} \leq M^{FG}$. The set $\{A_1, \ldots, A_{M^{CG}}\}$ is the set of coarse-grained variables. The coarse-grained variables define a space $V = \mathbb{R}^{M^{CG}}$ which we call the coarse-grained space. In general, any subset of functions can be chosen to be coarse-grained variables; however, as we will see later, a convenient choice is to select a subset of coordinates obtained via a *canonical transformation* of the Hamiltonian system.

We are now in the position to define the projection operator. Given a phase function $B$, we define the projection operator over the CG space as:

$$\mathcal{P}_{\mathbf{a}}B = \int_{A^{-1}(\{\mathbf{a}\})} B(\boldsymbol{\gamma})\mu_{\mathbf{a}}(\mathrm{d}\boldsymbol{\gamma})$$

where $A^{-1}(\{\mathbf{a}\})$ is the preimage of $\boldsymbol{\Gamma} \in \mathbb{R}^{M^{CG}}$, and $\mu_{\mathbf{a}}$ is the measure which satisfies

$$\int_V \left(\int_{A^{-1}(\{\mathbf{a}\})} B(\boldsymbol{\gamma})\mu_{\mathbf{a}}(\mathrm{d}\boldsymbol{\gamma})\right)\mathrm{d}\mathbf{a} = \int_X B(\boldsymbol{\gamma})\mu(\mathrm{d}\boldsymbol{\gamma})$$

for any integrable phase function $B$. If we interpret the phase functions as random variables, the projection operator has a nice interpretation as a conditional expectation over the coarse-grained variables:

$$\mathcal{P}_{\mathbf{a}} B = \mathbb{E}\left[B \,|\mathbf{A}(\boldsymbol{\gamma}) = \mathbf{a}\right]. \tag{S.5}$$

In the following we will write $\mathbb{E}\left[B|\mathbf{a}\right]$ as a condensed notation for the right–hand side of eq. (S.5). Given phase functions $B_i(\boldsymbol{\gamma})$ (we use subscripts when we need to distinguish between different phase functions only) the conditional expectation satisfy the following properties [2]:

- $\mathbb{E}\left[B|\mathbf{a}\right]$ is a function of $\mathbf{a}$;
- $\mathbb{E}\left[B|\mathbf{a}\right]$ is a linear operator on phase functions, i.e.

$$\mathbb{E}\left[\alpha B_1 + \gamma B_2|\mathbf{a}\right] = \alpha\mathbb{E}\left[B_1|\mathbf{a}\right] + \gamma\mathbb{E}\left[B_2|\mathbf{a}\right];$$

- $\mathbb{E}\left[B|\mathbf{a}\right]$ represents the best approximation of $B$ by a function of $\mathbf{a}$, i.e.

$$\mathbb{E}\left[\left|B - \mathbb{E}\left[B|\mathbf{a}\right]\right|^2\right] \leq \mathbb{E}\left[\left|B - f(\mathbf{a})\right|^2\right]$$

  for all phase functions $f$; $\mathcal{P}_{\mathbf{a}} = \mathbb{E}\left[B|\mathbf{a}\right]$ is therefore an orthogonal projection.

- For any function $f$ depending only on the value of $B_1$, i.e. $f(\boldsymbol{\gamma}) = g(B_1(\boldsymbol{\gamma}))$, for some $g$, we have

$$\mathbb{E}\left[\left(B - \mathbb{E}\left[B|\mathbf{a}\right]\right) f\right] = 0 \quad \text{and} \quad \mathbb{E}\left[f\, B_2|\mathbf{a}\right] = g(\mathbf{a})\mathbb{E}\left[B_2|\mathbf{a}\right] \tag{S.6}$$

The complementary orthogonal projection $\mathcal{Q}_{\mathbf{a}}$ is defined as

$$\mathcal{Q}_{\mathbf{a}} B(\boldsymbol{\gamma}) = B(\boldsymbol{\gamma}) - \mathcal{P}_{\mathbf{a}} B(\boldsymbol{\gamma}). \tag{S.7}$$

## II. EQUATION 6

Here, we give the derivation of the Generalized Langevin Equation in the main paper eq. (6). We start from eq. (2):

$$\frac{\partial \boldsymbol{\Gamma}(\boldsymbol{\gamma}(t))}{\partial t} = \mathfrak{L}\boldsymbol{\Gamma}(\boldsymbol{\gamma}(t)), \quad \boldsymbol{\Gamma}(\boldsymbol{\gamma}(0)) = \boldsymbol{\Gamma}(\boldsymbol{\gamma}_0). \tag{S.8}$$

By using the operator identity: $\mathcal{I} = \mathcal{P} + \mathcal{Q}$, and the following expression obtained by the solution of eq. (S.8) (eq. (3) of the main paper):

$$\mathfrak{L}\boldsymbol{\Gamma}(\boldsymbol{\gamma}(t)) = \mathfrak{L}\mathbf{e}^{t\mathfrak{L}}\boldsymbol{\Gamma}(\boldsymbol{\gamma}_0) = \mathbf{e}^{t\mathfrak{L}}\mathfrak{L}\boldsymbol{\Gamma}_0 \tag{S.9}$$

where $\boldsymbol{\Gamma}_0 = \boldsymbol{\Gamma}(\boldsymbol{\gamma})$. We can then rewrite the equation eq. (S.8) as:

$$\frac{\partial \boldsymbol{\Gamma}_t}{\partial t} = \mathbf{e}^{t\mathfrak{L}}(\mathcal{P} + \mathcal{Q})\mathfrak{L}\boldsymbol{\Gamma}_0 = \mathbf{e}^{t\mathfrak{L}}\mathcal{P}\mathfrak{L}\boldsymbol{\Gamma}_0 + \mathbf{e}^{t\mathfrak{L}}\mathcal{Q}\mathfrak{L}\boldsymbol{\Gamma}_0 \tag{S.10}$$

Now we use the Dunhamel-Dyson operator identity [3]:

$$\mathbf{e}^{t\mathfrak{L}} = \mathbf{e}^{t\mathcal{Q}\mathfrak{L}} + \int_0^t \mathbf{e}^{(t-s)\mathfrak{L}}\mathcal{P}\mathfrak{L}\mathbf{e}^{s\mathcal{Q}\mathfrak{L}}\,\mathrm{d}s \tag{S.11}$$

to rewrite the second term on the RHS of eq. (S.10) as

$$\mathbf{e}^{t\mathfrak{L}}\mathcal{Q}\mathfrak{L}\boldsymbol{\Gamma}_0 = \mathbf{e}^{t\mathcal{Q}\mathfrak{L}}\mathcal{Q}\mathfrak{L}\boldsymbol{\Gamma}_0 + \int_0^t \mathbf{e}^{(t-s)\mathfrak{L}}\mathcal{P}\mathfrak{L}\mathbf{e}^{s\mathcal{Q}\mathfrak{L}}\mathcal{Q}\mathfrak{L}\boldsymbol{\Gamma}_0\mathrm{d}s \tag{S.12}$$

We now consider the latter part of the integrand in eq. (S.12): [4]

$$
\begin{aligned}
\mathcal{P}\mathfrak{L}\mathbf{e}^{s\mathcal{Q}\mathfrak{L}}\mathcal{Q}\mathfrak{L}\mathbf{\Gamma}_0 &= \frac{1}{\Omega(\mathbf{a})}\int \delta\left(\mathbf{\Gamma}(\boldsymbol{\gamma})-\mathbf{a}\right)\mathfrak{L}\mathbf{e}^{s\mathcal{Q}\mathfrak{L}}\mathcal{Q}\mathfrak{L}\mathbf{\Gamma}_0\,\mu(\mathrm{d}\boldsymbol{\gamma})\\
&= -\frac{1}{\Omega(\mathbf{a})}\int \mathbf{e}^{s\mathcal{Q}\mathfrak{L}}\mathcal{Q}\mathfrak{L}\mathbf{\Gamma}_0\;\mathfrak{L}\delta\left(\mathbf{\Gamma}(\boldsymbol{\gamma})-\mathbf{a}\right)\mu(\mathrm{d}\boldsymbol{\gamma})
\end{aligned}
$$

where we used the fact that $\mathfrak{L}$ is skew–symmetric on $L^2(X;\mu)$. An application of the chain rule then gives

$$
\mathfrak{L}\delta\left(\mathbf{\Gamma}(\boldsymbol{\gamma})-\mathbf{a}\right)=\mathfrak{L}\mathbf{\Gamma}\cdot\nabla_{\mathbf{\Gamma}}\delta\left(\mathbf{\Gamma}(\boldsymbol{\gamma})-\mathbf{a}\right)=-\mathfrak{L}\mathbf{\Gamma}\cdot\nabla_{\mathbf{a}}\delta\left(\mathbf{\Gamma}(\boldsymbol{\gamma})-\mathbf{a}\right),
$$

where $\nabla_{\mathbf{x}}$ denotes the gradient taken with respect to the variable $\mathbf{x}$. We may now write

$$
\begin{aligned}
&-\frac{1}{\Omega(\mathbf{a})}\int \left[\mathbf{e}^{s\mathcal{Q}\mathfrak{L}}\mathcal{Q}\mathfrak{L}\mathbf{\Gamma}_0\right]\mathfrak{L}\delta\left(\mathbf{\Gamma}(\boldsymbol{\gamma})-\mathbf{a}\right)\mu(\mathrm{d}\boldsymbol{\gamma})\\
&\quad= -\frac{1}{\Omega(\mathbf{a})}\int \left[\mathbf{e}^{s\mathcal{Q}\mathfrak{L}}\mathcal{Q}\mathfrak{L}\mathbf{\Gamma}_0\right]\mathfrak{L}\mathbf{\Gamma}_0\cdot\nabla_{\mathbf{\Gamma}}\delta\left(\mathbf{\Gamma}(\boldsymbol{\gamma})-\mathbf{a}\right)\mu(\mathrm{d}\boldsymbol{\gamma})\\
&\quad= \frac{1}{\Omega(\mathbf{a})}\mathrm{Div}_{\mathbf{a}}\left(\int \mathbf{e}^{s\mathcal{Q}\mathfrak{L}}\mathcal{Q}\mathfrak{L}\mathbf{\Gamma}_0\otimes\mathfrak{L}\mathbf{\Gamma}_0\delta\left(\mathbf{\Gamma}(\boldsymbol{\gamma})-\mathbf{a}\right)\mu(\mathrm{d}\boldsymbol{\gamma})\right)\\
&\quad= \frac{1}{\Omega(\mathbf{a})}\mathrm{Div}_{\mathbf{a}}\left(\mathcal{P}\left(\mathbf{e}^{s\mathcal{Q}\mathfrak{L}}\mathcal{Q}\mathfrak{L}\mathbf{\Gamma}_0\otimes\mathfrak{L}\mathbf{\Gamma}_0\right)\Omega(\mathbf{a})\right)\\
&\quad= \mathcal{P}\left(\mathbf{e}^{s\mathcal{Q}\mathfrak{L}}\mathcal{Q}\mathfrak{L}\mathbf{\Gamma}_0\otimes\mathfrak{L}\mathbf{\Gamma}_0\right)\frac{\nabla_{\mathbf{a}}\Omega(\mathbf{a})}{\Omega(\mathbf{a})}+\mathrm{Div}_{\mathbf{a}}\mathcal{P}\left(\mathbf{e}^{s\mathcal{Q}\mathfrak{L}}\mathcal{Q}\mathfrak{L}\mathbf{\Gamma}_0\otimes\mathfrak{L}\mathbf{\Gamma}_0\right)\\
&\quad= -\mathcal{M}(\mathbf{a},s)\nabla_{\mathbf{a}}\mathcal{S}(\mathbf{a})+\beta^{-1}\mathrm{Div}_{\mathbf{a}}\mathcal{M}(\mathbf{a},s)
\end{aligned}
\tag{S.13}
$$

where $\mathrm{Div}_{\mathbf{a}}$ is the usual vector or matrix divergence taken with respect to the variable $\mathbf{a}$, and we have defined the free energy $\mathcal{S}$ and memory matrix $\mathcal{M}$:

$$
\begin{aligned}
\mathcal{S}(\mathbf{a}) &:= -\frac{1}{\beta}\ln\Omega(\mathbf{a})\\
\mathcal{M}(\mathbf{a},s) &= \beta\,\mathcal{P}\left(\mathbf{e}^{s\mathcal{Q}\mathfrak{L}}\mathcal{Q}\mathfrak{L}\mathbf{\Gamma}_0\otimes\mathcal{Q}\mathfrak{L}\mathbf{\Gamma}_0\right)=\beta\,\mathcal{P}\left(\boldsymbol{\mathcal{F}}(s,\boldsymbol{\gamma})\otimes\boldsymbol{\mathcal{F}}(0,\boldsymbol{\gamma})\right)
\end{aligned}
\tag{S.14}
$$

The fact that we may replace $\mathfrak{L}$ by $\mathcal{Q}\mathfrak{L}$ in the second term of the tensor product in order to pass to the last line in eq. (S.13) is a consequence of eq. (S.6):

$$
\begin{aligned}
\mathcal{P}\left(\mathbf{e}^{s\mathcal{Q}\mathfrak{L}}\mathcal{Q}\mathfrak{L}\mathbf{\Gamma}_0\otimes\mathfrak{L}\mathbf{\Gamma}_0\right) &= \mathcal{P}\left(\mathbf{e}^{s\mathcal{Q}\mathfrak{L}}\mathcal{Q}\mathfrak{L}\mathbf{\Gamma}_0\otimes\mathcal{P}\mathfrak{L}\mathbf{\Gamma}_0\right)+\mathcal{P}\left(\mathbf{e}^{s\mathcal{Q}\mathfrak{L}}\mathcal{Q}\mathfrak{L}\mathbf{\Gamma}_0\otimes\mathcal{Q}\mathfrak{L}\mathbf{\Gamma}_0\right)\\
&= \mathcal{P}\left(\mathbf{e}^{s\mathcal{Q}\mathfrak{L}}\mathcal{Q}\mathfrak{L}\mathbf{\Gamma}_0\right)\otimes\mathcal{P}\mathfrak{L}\mathbf{\Gamma}_0+\mathcal{P}\left(\mathbf{e}^{s\mathcal{Q}\mathfrak{L}}\mathcal{Q}\mathfrak{L}\mathbf{\Gamma}_0\otimes\mathcal{Q}\mathfrak{L}\mathbf{\Gamma}_0\right);
\end{aligned}
$$

the first term then vanishes since $\mathcal{P}\mathcal{Q}=0$.

Now, since $\mathbf{e}^{t\mathfrak{L}}f(\mathbf{\Gamma}(\gamma_0))=f(\mathbf{\Gamma}(\boldsymbol{\gamma}(t)))$, the terms in eq. (S.14) become:

$$
\begin{aligned}
\mathbf{e}^{t\mathfrak{L}}\mathcal{P}_{\mathbf{a}}\mathfrak{L}\mathbf{\Gamma} &= \mathcal{P}_{\mathbf{a}(t)}\mathfrak{L}\mathbf{\Gamma},\\
\mathbf{e}^{(t-s)\mathfrak{L}}\mathcal{M}(\mathbf{a},s)\nabla_{\mathbf{a}}\mathcal{S}(\mathbf{a}) &= \mathcal{M}(\mathbf{a}(t-s),s)\nabla_{\mathbf{a}}\mathcal{S}(\mathbf{a}(t-s)),\\
\mathbf{e}^{(t-s)\mathfrak{L}}\mathrm{Div}_{\mathbf{a}}\mathcal{M}(\mathbf{a},s) &= \mathrm{Div}_{\mathbf{a}}\mathcal{M}(\mathbf{a}(t-s),s),
\end{aligned}
$$

which completes the derivation.

## III. EQUATION 8

The eq. (8), which we report here:

$$
\boldsymbol{\mathcal{R}}(t,\boldsymbol{\gamma})=\mathbf{e}^{t\mathcal{Q}_{\mathbf{A}(\boldsymbol{\gamma})}}\mathcal{Q}_{\mathbf{A}(\boldsymbol{\gamma})}\mathfrak{L}\mathbf{A}(\boldsymbol{\gamma})
\tag{S.15}
$$

can be interpreted as a random force because it is uncorrelated with the projected variables. The proof of the last statement is based on the use of the Mori projector, which is a particular case of the Zwanzig projector when the system is near equilibrium [5] . By using the definition of scalar product in the Hilbert space of dynamic quantities (i.e. the observables) we can define the Mori projector $\mathcal{P}^M$ of a function $B(\boldsymbol{\gamma})$ in the direction of $A(\boldsymbol{\gamma})$ as:

$$\mathcal{P}^M B(\boldsymbol{\gamma}) = \frac{(B(\boldsymbol{\gamma}), A^{\star}(\boldsymbol{\gamma}))}{(A(\boldsymbol{\gamma}), A^{\star}(\boldsymbol{\gamma}))} A(\boldsymbol{\gamma}) \tag{S.16}$$

where $A^{\star}$ is the conjugate complement of $A$. The complement of $\mathcal{P}^M$, the projection of $B(\boldsymbol{\gamma}(t))$ in the direction perpendicular to $A(\boldsymbol{\gamma}(0)) = A(\boldsymbol{\gamma})$, $\mathcal{Q}^M$ can be written as:

$$\mathcal{Q}^M B(\boldsymbol{\gamma}(t)) = B(\boldsymbol{\gamma}(t)) - \frac{(B(\boldsymbol{\gamma}(t)), A^{\star}(\boldsymbol{\gamma}))}{(A(\boldsymbol{\gamma}), A^{\star}(\boldsymbol{\gamma}))} A(\boldsymbol{\gamma}) \tag{S.17}$$

If we now consider S.15 we can write:

$$\begin{aligned}
(\boldsymbol{\mathcal{F}}(t, \boldsymbol{\gamma}), A^{\star}(\boldsymbol{\gamma})) &= \left(\mathbf{e}^{t\mathcal{Q}^M_{A(\boldsymbol{\gamma})}} \mathcal{Q}^M_{A(\boldsymbol{\gamma})} \mathfrak{L} A(\boldsymbol{\gamma}), A^{\star}(\boldsymbol{\gamma})\right) \\
&= \left(\mathcal{Q}^M \mathbf{e}^{t\mathcal{Q}^M_{\mathbf{A}(\boldsymbol{\gamma})}} \mathcal{Q}_{\mathbf{A}(\boldsymbol{\gamma})} \mathfrak{L} A(\boldsymbol{\gamma}), A^{\star}\right) \\
&= \left(\mathcal{Q}^M \boldsymbol{\mathcal{R}}(t, \boldsymbol{\gamma}), A^{\star}(\boldsymbol{\gamma})\right) \\
&= \left((\boldsymbol{\mathcal{F}}(t, \boldsymbol{\gamma}), A^{\star}(\boldsymbol{\gamma})) - \frac{(\boldsymbol{\mathcal{F}}(t, \boldsymbol{\gamma}), A^{\star}(\boldsymbol{\gamma}))}{(A(\boldsymbol{\gamma}), A^{\star}(\boldsymbol{\gamma}))} (A(\boldsymbol{\gamma}), A^{\star}(\boldsymbol{\gamma}))\right) = 0
\end{aligned} \tag{S.18}$$

where we used the idempotent property of the projector. In the Langevin description of the dynamics of a system, the random force has the property of being uncorrelated from the velocity of the particle. For the same reason, being the dynamic of $\boldsymbol{\mathcal{F}}(t, \boldsymbol{\gamma})$ orthogonal to that of $A$ (i.e. they are uncorrelated) we can identify it as the random force acting on the system.

## IV. EQUATION 16

Integrals involving beads can be solved separately. Therefore we show the derivation for a single bead, the generalization for $N^B$ beads is straightforward. We start the derivation by rewriting the kinetic energy $K$ term of the $s^I$ atoms belonging to a generic bead $I$ in the Hamiltonian (eq. (10)) as:

$$K = \frac{\Phi_I^2}{2m_I} + \sum_{j=1}^{s_I - 1} \frac{\mathbf{k}_j^2}{2\nu_j} \tag{S.19}$$

where $\mathbf{P} = \Phi_I(\mathbf{p})$ and $\mathbf{k}_j$ are $s_I - 1$ fictitious particles with mass $\nu_j$ associated to relative motion of atoms within the bead, we dropped the dependence from $\mathbf{p}$ for clarity. We use the convention described in section III of the main paper, lower case letters represent phase space variables in FG system, capital letters represent position and momenta of CG particles.

The integral in eq. (16) can be rewritten as

$$k_B \log \frac{1}{\mathcal{Z}} \int \mathrm{d}\mathbf{p}_1 \cdots \mathrm{d}\mathbf{p}_{s_I} |\mathbf{J}| \ \exp\left[-\beta\left(\frac{\mathbf{P}_I^2}{2M_I} + \sum_{j=1}^{s_I - 1} \frac{\mathbf{k}_j^2}{2\nu_j}\right)\right] \delta\left(\Phi_I - \mathbf{P}_I\right) \tag{S.20}$$

Last step of the calculation involve change of integration variables in the previous integral. The change of variable needs the Jacobian $|\mathbf{J}|$, defined as the determinant of the Jacobian matrix of the change of variables $\mathbf{J} = \left(\frac{\partial \mathbf{P}, \mathbf{k}_1, \ldots, \mathbf{k}_{s_I - 1}}{\partial \mathbf{p}_1, \ldots, \mathbf{p}_{s_I}}\right)$.

The transformation involved are all linear in the old variables. Therefore, every entry in the Jacobian matrix is constant and the Jacobian is a constant quantity. We can write:

$$
\begin{aligned}
&k_B \log \frac{1}{\mathcal{K}} \int \mathrm{d}\mathbf{P}_I \mathrm{d}\mathbf{k}_1 \cdots \mathrm{d}\mathbf{k}_{s_I-1} |\mathbf{J}| \exp\left[-\beta \frac{\Phi_I^2}{2m_I}\right] \exp\left[-\beta \sum_{j=1}^{s_I-1} \frac{\mathbf{k}_j^2}{2\nu_j}\right] \delta\left(\Phi_I - \mathbf{P}_I\right) = \\
&\quad k_B \log\left(\frac{1}{\int \mathrm{d}\mathbf{P}_I \exp\left[-\beta \frac{\Phi_I^2}{2m_I}\right]} \int \mathrm{d}\Phi_I \exp\left[-\beta \frac{\Phi_I^2}{2m_I}\right] \delta\left(\Phi_I - \mathbf{P}_I\right)\right) + k_B \log\left(|\mathbf{J}|\right) \\
&\quad + k_B \log\left(\frac{1}{\int \mathrm{d}\mathbf{k}_1 \cdots \mathrm{d}\mathbf{k}_{s_I-1} \exp\left[-\beta \sum_{j=1}^{s_I-1} \frac{\mathbf{k}_j^2}{2\nu_j}\right]} \int \mathrm{d}\mathbf{k}_1 \cdots \mathrm{d}\mathbf{k}_{s_I-1} \exp\left[-\beta \sum_{j=1}^{s_I-1} \frac{\mathbf{k}_j^2}{2\nu_j}\right]\right) = \\
&\quad -\frac{1}{T} \frac{\mathbf{P}_I^2}{2m_I} - k_B \log\left(\sqrt{\frac{2\pi m_I}{\beta}}\right) + k_B \log\left(|\mathbf{J}|\right)
\end{aligned}
\tag{S.21}
$$

The second and third terms on the last equality are constant and can be ignored. The quantity $S$ appears in the GLE only as derivative of the new variables, therefore all constant quantities become null in eq. (6)

## V. EQUATION 19

$$
\begin{aligned}
-\frac{\partial V^{\text{eff}}}{\partial \mathbf{R}_J} &= \frac{\partial}{\partial \mathbf{R}_J} \left[ k_B T \log\left( \int \mathrm{d}\boldsymbol{\gamma}'_{\mathbf{r}} \frac{1}{\mathcal{Z}_{\mathbf{R},\mathbf{r}}} \mathbf{e}^{-\beta\left(U^{AB}(\mathbf{r},\hat{\mathbf{r}}') + U^{BB}(\hat{\mathbf{r}}')\right)} \prod_{K=1}^{M^{CG}} \delta\left(\Psi_K(\hat{\mathbf{r}}') - \mathbf{R}_K\right) \right) \right] \\
&= k_B T \frac{\frac{\partial}{\partial \mathbf{R}_J} \left( \int \mathrm{d}\boldsymbol{\gamma}'_{\mathbf{r}} \frac{1}{\mathcal{Z}_{\mathbf{R}}} \mathbf{e}^{-\beta\left(U^{AB}(\mathbf{r},\hat{\mathbf{r}}') + U^{BB}(\hat{\mathbf{r}}')\right)} \prod_{K=1}^{M^{CG}} \delta\left(\Psi_K(\hat{\mathbf{r}}') - \mathbf{R}_K\right) \right)}{\left( \int \mathrm{d}\boldsymbol{\gamma}'_{\mathbf{r}} \frac{1}{\mathcal{Z}_{\mathbf{R}}} \mathbf{e}^{-\beta(U^{AB}(\mathbf{r},\hat{\mathbf{r}}') + U^{BB}(\hat{\mathbf{r}}'))} \prod_{J=1}^{M^{CG}} \delta\left(\Psi_J(\hat{\mathbf{r}}') - \mathbf{R}_J\right) \right)}
\end{aligned}
\tag{S.22}
$$

We can write for the numerator:

$$\frac{\partial}{\partial \mathbf{R}_J}\left(\int \mathrm{d}\boldsymbol{\gamma}'_{\mathbf{r}} \frac{1}{\mathcal{Z}_{\mathbf{R}}} \mathbf{e}^{-\beta\left(U^{AB}(\mathbf{r},\hat{\mathbf{r}}')+U^{BB}(\hat{\mathbf{r}}')\right)} \prod_{K=1}^{M^{CG}} \delta\left(\Psi_K(\hat{\mathbf{r}}') - \mathbf{R}_K\right)\right)$$

$$= -\int \mathrm{d}\boldsymbol{\gamma}'_{\mathbf{r}} \frac{1}{\mathcal{Z}_{\mathbf{R}}} \mathbf{e}^{-\beta\left(U^{AB}(\mathbf{r},\hat{\mathbf{r}}')+U^{BB}(\hat{\mathbf{r}}')\right)} \frac{\partial}{\partial \Psi_J} \delta\left(\Psi_J(\hat{\mathbf{r}}') - \mathbf{R}_J\right) \prod_{\substack{K=1\\K\neq J}}^{M^{CG}} \delta\left(\Psi_K(\hat{\mathbf{r}}') - \mathbf{R}_K\right)$$

$$= -\int \mathrm{d}\boldsymbol{\gamma}'_{\mathbf{r}} \frac{1}{\mathcal{Z}_{\mathbf{R}}} \mathbf{e}^{-\beta\left(U^{AB}(\mathbf{r},\hat{\mathbf{r}}')+U^{BB}(\hat{\mathbf{r}}')\right)} \sum_{i=1}^{s_J} \frac{1}{c_{J_i} s_J} \frac{\partial}{\partial \mathbf{r}_{J_i}} \delta\left(\Psi_J(\hat{\mathbf{r}}') - \mathbf{R}_J\right) \prod_{\substack{K=1\\K\neq J}}^{M^{CG}} \delta\left(\Psi_K(\hat{\mathbf{r}}') - \mathbf{R}_K\right)$$

$$= \int \mathrm{d}\boldsymbol{\gamma}'_{\mathbf{r}} \frac{1}{\mathcal{Z}_{\mathbf{R}}} \sum_{i=1}^{s_J} \frac{1}{c_{J_i} s_J} \frac{\partial}{\partial \mathbf{r}_{J_i}} \mathbf{e}^{-\beta\left(U^{AB}(\mathbf{r},\hat{\mathbf{r}}')+U^{BB}(\hat{\mathbf{r}}')\right)} \prod_{\substack{K=1\\K\neq J}}^{M^{CG}} \delta\left(\Psi_K(\hat{\mathbf{r}}') - \mathbf{R}_K\right)$$

$$= \beta \int \mathrm{d}\boldsymbol{\gamma}'_{\mathbf{r}} \frac{1}{\mathcal{Z}_{\mathbf{R}}} \left[\sum_{i=1}^{s_J} \frac{1}{c_{J_i} s_J} \left(-\frac{\partial}{\partial \mathbf{r}_{J_i}} \left(U^{AB}(\mathbf{r},\hat{\mathbf{r}}') + U^{BB}(\hat{\mathbf{r}}')\right)\right)\right] \mathbf{e}^{-\beta\left(U^{AB}(\mathbf{r},\hat{\mathbf{r}}')+U^{BB}(\hat{\mathbf{r}}')\right)}$$
$$\prod_{\substack{K=1\\K\neq J}}^{M^{CG}} \delta\left(\Psi_K(\hat{\mathbf{r}}') - \mathbf{R}_K\right)$$

$$= \beta \int \mathrm{d}\boldsymbol{\gamma}'_{\mathbf{r}} \frac{1}{\mathcal{Z}_{\mathbf{R}}} \left[\sum_{i=1}^{s_J} \frac{1}{c_{J_i} s_J} \mathbf{F}_{J_i}\right] \mathbf{e}^{-\beta\left(U^{AB}(\mathbf{r},\hat{\mathbf{r}}')+U^{BB}(\hat{\mathbf{r}}')\right)} \tag{S.23}$$

where $\mathbf{F}_{J_i}$ is the force acting on the $i$-th atom of the $J$-th bead. We define $\mathbf{F}_J = \sum_{i=1}^{s_J} \frac{1}{c_{J_i} s_J} \mathbf{F}_{J_i}$ as the weighted force on the $J$-th bead. We used the following proprieties of Dirac $\delta$-function valid for a generic function of the phase-space $f(\boldsymbol{\gamma})$:

$$\int \mathrm{d}\boldsymbol{\gamma}'_{\mathbf{r}} f(\boldsymbol{\gamma}) \frac{\partial}{\partial \boldsymbol{\gamma}} \delta\left(\boldsymbol{\gamma}'_{\mathbf{r}} - \boldsymbol{\gamma}\right) = -\int \mathrm{d}\boldsymbol{\gamma}'_{\mathbf{r}} \frac{\partial f(\boldsymbol{\gamma})}{\partial \boldsymbol{\gamma}} \delta\left(\boldsymbol{\gamma}'_{\mathbf{r}} - \boldsymbol{\gamma}\right) = -\int \mathrm{d}\boldsymbol{\gamma}'_{\mathbf{r}} f(\boldsymbol{\gamma}) \frac{\partial}{\partial \boldsymbol{\gamma}'_{\mathbf{r}}} \delta\left(\boldsymbol{\gamma}'_{\mathbf{r}} - \boldsymbol{\gamma}\right)$$

and the fact that

$$\int \mathrm{d}\boldsymbol{\gamma}'_{\mathbf{r}} f(\boldsymbol{\gamma}) \frac{\partial}{\partial \Psi_J} \delta\left(\Psi_J(\hat{\mathbf{r}}') - \mathbf{R}_J\right) = \int \mathrm{d}\boldsymbol{\gamma}'_{\mathbf{r}} f(\boldsymbol{\gamma}) \frac{\partial \mathbf{r}'_{J_i}}{\partial \Psi_J} \frac{\partial}{\partial \mathbf{r}'_{J_i}} \delta\left(\Psi_J(\hat{\mathbf{r}}') - \mathbf{R}_J\right) \tag{S.24}$$

and by summing over $s_J$

$$\int \mathrm{d}\boldsymbol{\gamma}'_{\mathbf{r}} f(\boldsymbol{\gamma}) s_J \frac{\partial}{\partial \Psi_J} \delta\left(\Psi_J(\hat{\mathbf{r}}') - \mathbf{R}_J\right) = \int \mathrm{d}\boldsymbol{\gamma}'_{\mathbf{r}} f(\boldsymbol{\gamma}) \sum_{i=1}^{s_J} \frac{1}{c_{J_i}} \frac{\partial}{\partial \mathbf{r}'_{J_i}} \delta\left(\Psi_J(\hat{\mathbf{r}}') - \mathbf{R}_J\right) \tag{S.25}$$

By combining everything together we get eq. (19)

## VI. ORTHOGONAL DYNAMICS, EQUATION 28

In this section we give a derivation of the orthogonal dynamics defined in section V F of the paper. The starting point is the definition of the Lagrangian of the atomistic system, to which we impose the constraints. By using the standard theory of the action we derive the Hamiltonian equation for the constrained system.

The Lagrangian for the atomistic system is defined as:

$$\mathcal{L}(\dot{\boldsymbol{\gamma}}_{\mathbf{r}}, \boldsymbol{\gamma}_{\mathbf{r}}) = \frac{1}{2} \dot{\boldsymbol{\gamma}}_{\mathbf{r}}^{\mathrm{T}} \mathbf{M} \dot{\boldsymbol{\gamma}}_{\mathbf{r}} - U(\boldsymbol{\gamma}_{\mathbf{r}}) \tag{S.26}$$

where $\dot{\boldsymbol{\gamma}}_{\mathbf{r}}$ is the velocity vector, and we have defined $\mathbf{M}$ to be the diagonal mass matrix.

In the Lagrangian framework, constraining beads amounts to requiring that:

$$\sum_{i\in S_I}\frac{m_i}{M_I}\mathbf{r}_i=\mathbf{R}_i \tag{S.27}$$

for all $I=1,\ldots,M^{CG}$. Introducing the action functional $\mathfrak{S}$ involving the original Lagrangian eq. (S.26) and the constraints imposed with accompanying Lagrange multipliers, we have

$$\mathfrak{S}[\boldsymbol{\gamma}_{\mathbf{r}},\lambda]=\int_0^T \mathrm{d}t\left(\mathcal{L}(\dot{\boldsymbol{\gamma}}_{\mathbf{r}},\boldsymbol{\gamma}_{\mathbf{r}})+\sum_I\lambda_I\Big(\sum_{j\in S_I}\frac{m_j}{M_I}\mathbf{r}_j-\mathbf{R}_I\Big)\right)$$

The Lagrange multipliers $\lambda_I$ are functions of time, and we will use the principle of least action to derive the explicit form of the constraints to be used in the dynamic equations. If $\mathbf{r}(t)$ is the trajectory that minimizes the action, we vary by defining

$$\mathbf{r}(t;\sigma)\equiv\mathbf{r}(t)+\sigma\boldsymbol{\gamma}(t) \tag{S.28}$$

where $\sigma$ is a parameter and $\boldsymbol{\gamma}(t)$ is an arbitrary function with the requirement that it vanishes at the integration boundaries $\boldsymbol{\gamma}(0)=\boldsymbol{\gamma}(T)=0$. The parametric trajectory $\mathbf{r}(t;\sigma)$ equals the real trajectory $\mathbf{r}(t)$ when $\sigma=0$ and the time derivative is $\frac{\mathrm{d}}{\mathrm{d}t}\mathbf{r}(t;\sigma)=\dot{\mathbf{r}}(t)+\sigma\dot{\mathbf{X}}(t)$.

We now rewrite the action as function of the parametric trajectory as:

$$\mathfrak{S}[\boldsymbol{\gamma}_{\mathbf{r}}+\sigma\mathbf{X},\lambda,\mu]=\int_0^T\left(\mathcal{L}(\dot{\boldsymbol{\gamma}}_{\mathbf{r}}+\sigma\dot{\mathbf{X}},\boldsymbol{\gamma}_{\mathbf{r}}+\sigma\mathbf{X})+\sum_I\lambda_I\Big(\sum_{j\in S_I}\frac{m_j}{M_I}(\mathbf{r}_j+\sigma\mathbf{X}_j)-\mathbf{R}_I\Big)\right)\mathrm{d}t$$

Using the fact that $\sigma=0$ corresponds to an extremum of the action (by hypothesis), we must have that

$$0=\frac{\mathrm{d}\mathfrak{S}}{\mathrm{d}\sigma}\bigg|_{\sigma=0}=\int_0^T\mathrm{d}t\left(\nabla_{\dot{\mathbf{r}}}\mathcal{L}\cdot\dot{\mathbf{X}}+\nabla_{\mathbf{r}}\mathcal{L}\cdot\mathbf{X}+\sum_I\lambda_I\sum_{j\in S_I}\frac{m_j}{M_I}\mathbf{X}_j\right)$$

Integrating by parts, and using the fact that the function $\mathbf{X}$ is arbitary, we infer that

$$-m_i\ddot{\mathbf{r}}_i-\partial_{\mathbf{r}_i}U(\boldsymbol{\gamma}_{\mathbf{r}})+\lambda_I\frac{m_i}{M_I}=0\qquad\text{for all } i,\ \text{where } i\in S_I.$$

If $\mathbf{R}_I$ is constant in time, the constraints eq. (S.27) entail that

$$\sum_{i\in S_I}m_i\ddot{\mathbf{r}}_i=0,\quad\text{and thus}\quad\lambda_I=\sum_{i\in S_I}\frac{\partial U(\boldsymbol{\gamma}_{\mathbf{r}})}{\partial\mathbf{r}_i}.$$

Substituting the value obtained for $\lambda_I$, the resulting equations of motion can be written as:

$$\dot{\mathbf{r}}_j=\frac{\mathbf{p}_j}{m_j}\qquad\dot{\mathbf{p}}_j=-\frac{\partial U(\boldsymbol{\gamma}_{\mathbf{r}})}{\partial\mathbf{r}_j}+\frac{m_j}{M_I}\sum_{i\in S_I}\frac{\partial U(\boldsymbol{\gamma}_{\mathbf{r}})}{\partial\mathbf{r}_i}.$$

## VII. POLYNOMIAL INTERPOLATION FOR NOISY DATA

To approximate the value of a function at a point $\mathbf{x}$ by a polynomial of degree $N$, given noisy data points $\{(\mathbf{X}_i,\mathbf{Y}_i)\}_{i=1}^S$, the diagonal $S\times S$ Gaussian weight matrix $\mathbf{W}$, and the $S\times N$ Jacobian matrix $\mathbf{J}\in$ are formed, where

$$\mathbf{W}_{ij}=\begin{cases}\mathbf{e}^{-\frac{|\mathbf{x}-\mathbf{X}_i|^2}{\sigma^2}} & i=j,\\ 0 & \text{otherwise,}\end{cases}\quad\text{and}\quad\mathbf{J}_{ji}=(\mathbf{x}-\mathbf{X}_i)^{j-1}\quad\text{for } j=1,2,\ldots,N.$$

If $\mathbf{c}$ is the column vector of coefficients of a polynomial of degree $N$ approximating the data weighted by the Gaussian with standard deviation $\sigma$ with coordinates centred at $\mathbf{x}$, then $\mathbf{c}$ is a least squares solution to the equation

$$\mathbf{J}^T\mathbf{c} = \mathbf{Y},$$

with weight matrix $\mathbf{W}$. The first component of $\mathbf{c}$ is then the value of the function, and subsequent components are related to derivatives. In practice, we chose the parameter $\sigma = 0.1$ in our computations.

---


[1] Givon, D.; Hald, O. H.; Kupferman, R. Existence Proof for Orthogonal Dynamics and the Mori-Zwanzig Formalism. *Israel Journal of Mathematics* **2005**, *145*, 221–241.

[2] Chorin, A. J.; Hald, O. H.; Kupferman, R. Optimal prediction and the Mori-Zwanzig representation of irreversible processes. *PNAS* **2000**, *97*, 2968–2973.

[3] Evans, D.; Morris, G. *Statistical Mechanics of Nonequilibrium Liquids*; London: Academic, 1990.

[4] Hijòn, C.; Español, P.; Vanden-Eijnden, E.; R., D.-B. Mori–Zwanzig formalism as a practical computational tool. *Faraday Discussions* **2010**, *144*, 301–322.

[5] Kauzlarić, D.; Español, P.; Greiner, A.; Succi, S. Three Routes to the Friction Matrix and Their Application to the Coarse-Graining of Atomic Lattices. *Macromolecular Theory and Simulations* **2011**, *20*, 526–540.
